# Supplementary material for: Dynamic-Weighted Simplex Strategy for Learning Enabled Cyber Physical Systems
Source: arXiv:1902.02432 source file (2020-03-10)
Supplement: Supplementary file 1 [file appendix-text.tex]

% \begin{figure}[t]
% \centering
% \includegraphics[height=3cm, width=0.9\columnwidth]{figures/blurexample.PNG}
% \caption{The inverse relationship between the variance of Laplacian and the accuracy of the CNN predictor is shown. The original image (left) had an error of 0.19 degrees, the image blurred with a 5x5 Guassian filter (middle) had an error of 3.13 degrees, and the image blurred with a 7x7 filter (right) had an error of 5.54 degrees.}
% \label{fig:laplace}
% \end{figure}

\subsection{DeepNNCar Features}
Some additional features to aid the functioning of DeepNNCar are discussed below:

\subsubsection{Image Quality Analyzer}
To quantify the quality of the images captured by DeepNNCar, we used the variance of laplacian (as discussed in Literature \cite{PechPacheco2000DiatomAI}. In this approach, a laplacian kernel is convolved across the image, which computes the second derivative of the pixel intensities, from which the variance is calculated. A high variance value indicates an in-focus image whereas a low variance indicates an out of focus image.

To gain useful information from this technique, we systematically blurred sample images to find a threshold to determine if an image was in focus or not (Figure \ref{fig:laplace}). The threshold was tested by checking the error between the steering decision on the same location of track before the blur was applied and after the blur was applied. This was an offline mechanism we used to select good quality images for training the LEC model. 

\begin{figure}[t]
\centering
\setlength{\belowcaptionskip}{-10pt}
 \includegraphics[width=\columnwidth]{figures/wiring.pdf}
 \caption{The hardware wiring onboard DeepNNCar's motors and RPi3.}
 \label{fig:wiring}
 \vspace{-0.4em}
 \end{figure}

\subsubsection{2D Path Tracker}
To estimate the position vector of DeepNNCar, the speed of the car must be calculated, and this is accomplished using the IR-Optocoupler. The speed of DeepNNCar is calculated with the following equation: 

\begin{equation}
\lambda_t\times\pi\times d     
\end{equation}
 
Where, $\lambda_t$ is the frequency of interrupt generation and d is the diameter of the wheel. 

However, there are two constraints to this calculation: (1) the system must timeout and detect when the car is not moving, this is called as zero-detection time and is denoted as $T_{zd}$, and (2) the interrupt has a bounce time (time for switching between states) which is denoted as $T_{bt}$. Therefore, $\lambda$ is constrained by
$  \lambda_t \in [\frac{1}{T_{zd}},\frac{1}{T_{bt}}]
$ and any value that fall outside this range should be disregarded.

The heading of DeepNNCar is calculated by utilizing the direct relationship between the steering duty cycle [10,20] and the steering angle [-30\textdegree,30\textdegree]. The steering duty cycle computed is converted to angles and is used to project the trajectory of the car on a 2D map.  
The position vector $P_t = [P_x, P_y]$ is a function of the velocity vector $\nu_t = [\nu_x, \nu_y]$ and the new position is calculated as:

\begin{equation}
    P_{t+1} = P_t + \nu_t \cdot \Delta\\t
\end{equation}

Using this equation, the path of DeepNNCar is reconstructed in real-time, which is displayed on the dashboard of the client laptop (in Figure \ref{fig:ClientFeedback}).

\subsection{System Level Confidence Estimation}
\label{sec:CM}
\begin{figure}[t]
\centering
\includegraphics[height=3cm, width=0.9\columnwidth]{figures/blurexample.PNG}
\caption{The inverse relationship between the variance of Laplacian and the accuracy of the CNN predictor is shown. The original image (left) had an error of 0.19 degrees, the image blurred with a 5x5 Guassian filter (middle) had an error of 3.13 degrees, and the image blurred with a 7x7 filter (right) had an error of 5.54 degrees.}
\label{fig:laplace}
\vspace{-0.4em}
\end{figure}

\begin{table*}[t]
\centering
\footnotesize
\caption{Conditional Probability Table for \textit{SafeTurnRegion} node.}
\scalebox{0.8}{
\begin{tabular}{llllllllllllllllllllllllllll}
\hline
\multicolumn{1}{|l|}{\begin{tabular}[c]{@{}l@{}}Current\\ Position\end{tabular}} & \multicolumn{9}{l|}{Near} & \multicolumn{9}{l|}{On} & \multicolumn{9}{l|}{Far} \\ \hline
\multicolumn{1}{|l|}{\begin{tabular}[c]{@{}l@{}}Current\\ Velocity\end{tabular}} & \multicolumn{3}{l|}{Slow} & \multicolumn{3}{l|}{Medium} & \multicolumn{3}{l|}{Fast} & \multicolumn{3}{l|}{Slow} & \multicolumn{3}{l|}{Medium} & \multicolumn{3}{l|}{Fast} & \multicolumn{3}{l|}{Slow} & \multicolumn{3}{l|}{Medium} & \multicolumn{3}{l|}{Fast} \\ \hline
\multicolumn{1}{|l|}{\begin{tabular}[c]{@{}l@{}}Current\\ Steering\textsuperscript{*}\end{tabular}} & \multicolumn{1}{l|}{S} & \multicolumn{1}{l|}{L} & \multicolumn{1}{l|}{R} & \multicolumn{1}{l|}{S} & \multicolumn{1}{l|}{L} & \multicolumn{1}{l|}{R} & \multicolumn{1}{l|}{S} & \multicolumn{1}{l|}{L} & \multicolumn{1}{l|}{R} & \multicolumn{1}{l|}{S} & \multicolumn{1}{l|}{L} & \multicolumn{1}{l|}{R} & \multicolumn{1}{l|}{S} & \multicolumn{1}{l|}{L} & \multicolumn{1}{l|}{R} & \multicolumn{1}{l|}{S} & \multicolumn{1}{l|}{L} & \multicolumn{1}{l|}{R} & \multicolumn{1}{l|}{S} & \multicolumn{1}{l|}{L} & \multicolumn{1}{l|}{R} & \multicolumn{1}{l|}{S} & \multicolumn{1}{l|}{L} & \multicolumn{1}{l|}{R} & \multicolumn{1}{l|}{S} & \multicolumn{1}{l|}{L} & \multicolumn{1}{l|}{R} \\ \hline
\multicolumn{1}{|l|}{\begin{tabular}[c]{@{}l@{}}SafeTurnRegion\\ =Yes\end{tabular}} & \multicolumn{1}{l|}{1} & \multicolumn{1}{l|}{0.8} & \multicolumn{1}{l|}{0.8} & \multicolumn{1}{l|}{0.9} & \multicolumn{1}{l|}{0.6} & \multicolumn{1}{l|}{0.6} & \multicolumn{1}{l|}{0.2} & \multicolumn{1}{l|}{0.1} & \multicolumn{1}{l|}{0.1} & \multicolumn{1}{l|}{1} & \multicolumn{1}{l|}{1} & \multicolumn{1}{l|}{1} & \multicolumn{1}{l|}{1} & \multicolumn{1}{l|}{1} & \multicolumn{1}{l|}{1} & \multicolumn{1}{l|}{1} & \multicolumn{1}{l|}{1} & \multicolumn{1}{l|}{1} & \multicolumn{1}{l|}{0.9} & \multicolumn{1}{l|}{0.9} & \multicolumn{1}{l|}{0.9} & \multicolumn{1}{l|}{0.8} & \multicolumn{1}{l|}{0.7} & \multicolumn{1}{l|}{0.7} & \multicolumn{1}{l|}{0.5} & \multicolumn{1}{l|}{0.2} & \multicolumn{1}{l|}{0.2} \\ \hline
\multicolumn{1}{|l|}{\begin{tabular}[c]{@{}l@{}}SafeTurnRegion\\ =No\end{tabular}} & \multicolumn{1}{l|}{0} & \multicolumn{1}{l|}{0.2} & \multicolumn{1}{l|}{0.2} & \multicolumn{1}{l|}{0.1} & \multicolumn{1}{l|}{0.4} & \multicolumn{1}{l|}{0.4} & \multicolumn{1}{l|}{0.8} & \multicolumn{1}{l|}{0.9} & \multicolumn{1}{l|}{0.9} & \multicolumn{1}{l|}{0} & \multicolumn{1}{l|}{0} & \multicolumn{1}{l|}{0} & \multicolumn{1}{l|}{0} & \multicolumn{1}{l|}{0} & \multicolumn{1}{l|}{0} & \multicolumn{1}{l|}{0} & \multicolumn{1}{l|}{0} & \multicolumn{1}{l|}{0} & \multicolumn{1}{l|}{0.1} & \multicolumn{1}{l|}{0.1} & \multicolumn{1}{l|}{0.1} & \multicolumn{1}{l|}{0.2} & \multicolumn{1}{l|}{0.3} & \multicolumn{1}{l|}{0.3} & \multicolumn{1}{l|}{0.5} & \multicolumn{1}{l|}{0.8} & \multicolumn{1}{l|}{0.8} \\ \hline
\multicolumn{28}{c}{\textsuperscript{*} - Current Steering states : S=Straight, L=Left, R=Right.}
\end{tabular}
}
\label{tab:cpt1}
% \end{table*}
\vspace{4mm}
% \begin{table*}[t]
\centering
\footnotesize
\caption{Conditional Probability Table for \textit{InTrack} node }
\scalebox{0.9}{
\begin{tabular}{|l|l|l|l|l|l|l|l|l|l|l|l|l|l|l|l|l|l|l|}
\hline
SafeTurnRegion    & \multicolumn{9}{l|}{Yes}                                                               & \multicolumn{9}{l|}{No}                                                              \\ \hline
CmdSteering & \multicolumn{3}{l|}{Left} & \multicolumn{3}{l|}{Straight} & \multicolumn{3}{l|}{Right} & \multicolumn{3}{l|}{Left} & \multicolumn{3}{l|}{Straight} & \multicolumn{3}{l|}{Right} \\ \hline
Velocity  & Slow   & Med.   & Fast  & Slow    & Med.    & Fast    & Slow   & Med.   & Fast   & Slow   & Med.   & Fast  & Slow    & Med.    & Fast    & Slow   & Med.   & Fast   \\ \hline
InTrack=Y       & 0.6    & 0.2      & 0     & 0.7     & 0.5       & 0       & 1      & 0.9      & 0      & 0.2    & 0.1      & 0     & 0.3     & 0.2       & 0       & 0.5    & 0.4      & 0      \\ \hline
InTrack=N        & 0.4    & 0.8      & 1     & 0.3     & 0.5       & 1       & 0      & 0.1      & 1      & 0.8    & 0.9      & 1     & 0.7     & 0.8       & 1       & 0.5    & 0.6      & 1      \\ \hline
\end{tabular}
}
\label{tab:cpt2}
\end{table*}

\begin{figure*}[!ht] 
%   \label{ fig7} 
  \begin{minipage}[t][5cm][t]{\columnwidth}
    \centering
    \captionsetup{width=0.85\linewidth}
    \includegraphics[width=0.85\columnwidth]{figures/priors.png} 
    \caption{Bayesian Network model for Safety Assurance}
    \label{fig:BNModel}
  \end{minipage}%%
  \hfill
  \begin{minipage}[t][5cm][t]{\columnwidth}
    \centering
    \includegraphics[width=0.85\columnwidth]{figures/slow.png} 
    \captionsetup{width=0.85\linewidth}
    \caption{Bayesian Inference when \textit{current-velocity} is set to \textit{Slow}}
    \label{fig:bnslow}
  \end{minipage} 
  \vfill
  \begin{minipage}[t][5cm][t]{\columnwidth}
    \centering
    \includegraphics[width=0.85\columnwidth]{figures/fast.png} 
    \captionsetup{width=0.85\linewidth}
    \caption{Bayesian Inference when \textit{current-velocity} is set to \textit{Fast}}
    \label{fig:bnfast}
  \end{minipage}%% 
  \hfill
  \begin{minipage}[t][5cm][t]{\columnwidth}
    \centering
    \includegraphics[width=0.85\columnwidth]{figures/medium_far_straight.png} 
    \captionsetup{width=0.85\linewidth}
    \caption{Bayesian Inference when \textit{current-velocity} is set to \textit{Medium}, \textit{current-steering} is set to \textit{Straight} and \textit{current-position} is set to \textit{Far}} 
    \label{fig:bnmedium_near_straight}
  \end{minipage}
\end{figure*}

For autonomous systems, it is necessary to develop a mechanism that can monitor the system operation and provide a level of confidence as to how safe the system will be in different operating scenarios. This is difficult as it requires an effective knowledge of the distribution of the environment in which the system operates. In case of the DeepNNCar, we use a Bayesian Network model to estimate the probability that the car will remain on track, given its current state and control actions. 

Data collected during training and evaluation, is used to build a model to estimate the current position of the car. The data is also used to identify safe-turn regions (in different regions of the track) and the ranges for commands that keep the car within the track (at different speeds of operation). The nodes \textit{current-position}, \textit{current-velocity} and \textit{current-steering} capture the current state of the car. The node \textit{SafeTurnRegion} captures the likelihood of the car being in the safe-turn region when a control-cycle update is triggered. \textit{SafeTurnRegion} and the steering command \textit{CmdSteeringOnTurn} issued when the car is in the safe turn region influence the likelihood of the car remaining \textit{InTrack}. 

The \textit{current-position} node corresponds to the car distance from the next safe turn region. The discrete states based on the distance include \textit {On}, \textit{Near} and, \textit{Far}. The discrete states for \textit{current-velocity} are \textit{Slow} (less than 0.25 m/s), \textit{Medium} (between 0.25 and 0.6 m/s) and \textit{Fast} (greater than 0.6 m/s). The \textit{current-steering} node corresponds to the current steering angle of the car relative to its desired direction and includes the states \textit{left} (less than -10\textdegree), \textit{straight} (between -10\textdegree and +10\textdegree) and \textit{right} (greater than 10\textdegree). The node \textit{CmdSteeringOnTurn} corresponds to the steering command issued when the car is on the safe turn region and includes the states (\textit{Left}, \textit{Right} and \textit{Straight}) which are based on the range of the steering command values. The node \textit{InTrack} indicates if the car will remain on track when the turn is executed. This node include two states \textit{yes} and \textit{no}.

Tables \ref{tab:cpt1} and~\ref{tab:cpt2} capture the conditional probability tables for the  nodes \textit{SafeTurnRegion} and \textit{InTrack} respectively. The tables have been filled based on our understanding of the system during experimentation. The prior probabilities on the \textit{Current-Position} node shows that there is an equal chance of the car being in the three position states. With regards to \textit{Current-Steering}, the \textit{Left} state has a low probability due to the shape of the track and the nature of the mission. The \textit{Left} state is observed only when there is an error or there is a course correction for an error. The \textit{Current-Velocity} has been observed to be in the medium range most of the time giving the \textit{Medium} state a higher prior probability. The lower velocity states are observed in the beginning, while the fast speeds are not common. Given the shape of the track, the steering command during turns is mostly right as seen in the priors for \textit{CmdSteeringOnTurn}. 

Based on the priors for the root (observation) nodes and the likelihoods captured in the conditional probability tables, the priors for the assurance nodes (\textit{SafeTurnRegion} and \textit{InTrack}) can be inferred. The prior probability of being on track (0.7) reflects our experimental evidence with CSW-Simplex architecture. The Bayesian network model was used to compute the confidence metric that indicated the probability of car being in the turn region to execute control action under different situations. This was done by setting the evidence on the root (observation) nodes and executing the Bayesian inference engine to compute the posterior probabilities. 

The model predicts that when the \textit{current-velocity} is set to \textit{Slow}, there is a high probability of the car being in the safe turn region and remaining on the track (Figure \ref{fig:bnslow}). Alternately, figure \ref{fig:bnfast}, shows that when the speed is set to \textit{Fast}, the chance of being in the safe turn region to execute a control action is greatly reduced and there is no chance of remaining on the track.  Figure \ref{fig:bnmedium_near_straight} shows that when the \textit{current-velocity} is \textit{Medium}, \textit{current-steering} is \textit{Straight} and the \textit{current-position} is \textit{Far} from the safe turn region, there is a good chance of the car executing a control action in the safe turn region (80\%) and remaining on track (77\%). The results of the Bayesian Network agree with our experimental observations.
